# Supplementary material for: Semantics-Aware Image to Image Translation and Domain Transfer
Source: arXiv:1904.02203 source file (2021-03-01)

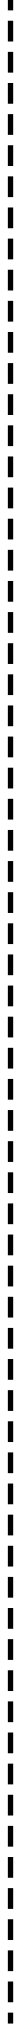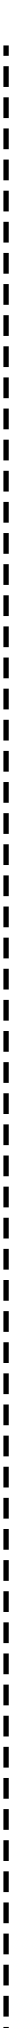



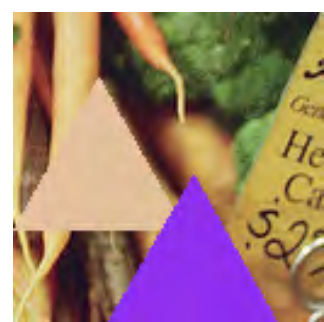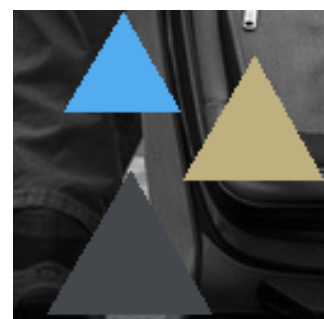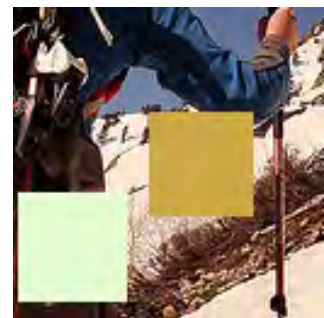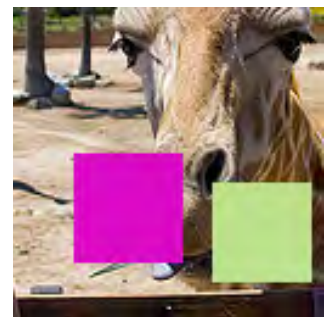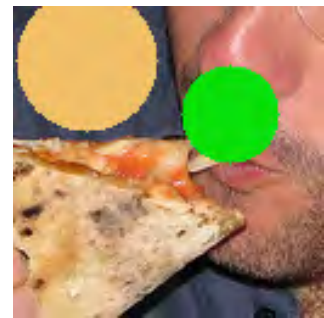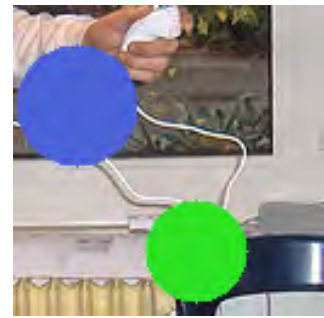

Supplement: Supplementary file 2 [file shapes_supp_qual_reverse.pdf]
