# Supplementary material for: Semantics-Aware Image to Image Translation and Domain Transfer
Source: arXiv:1904.02203 source file (2021-03-01)

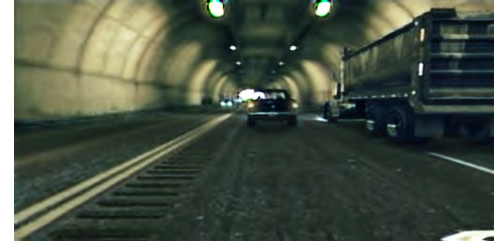

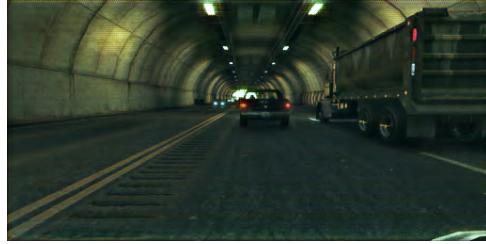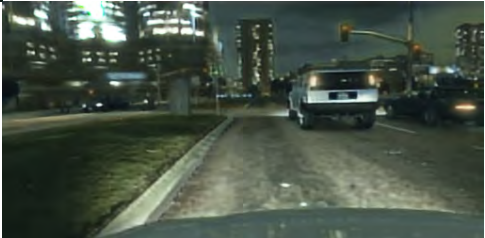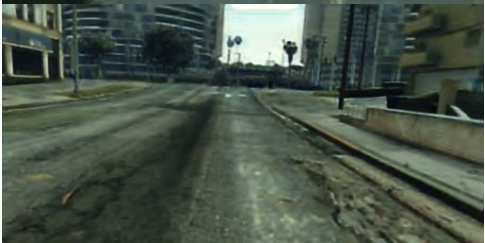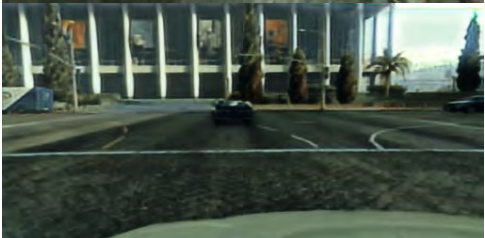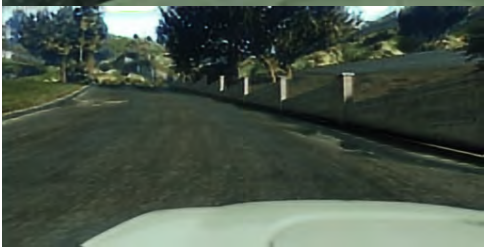

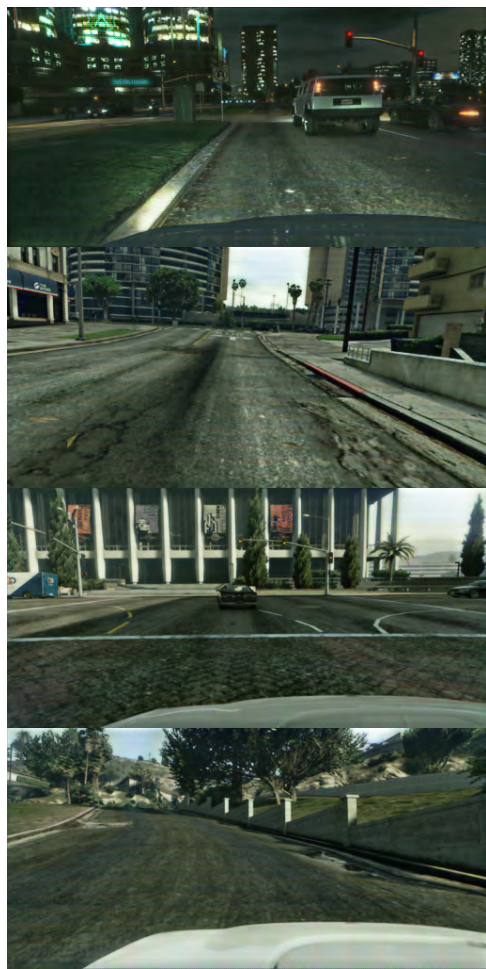

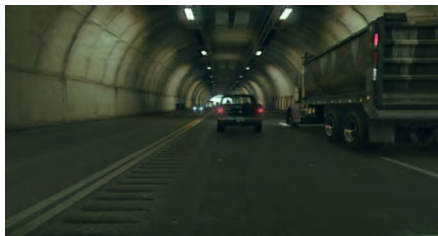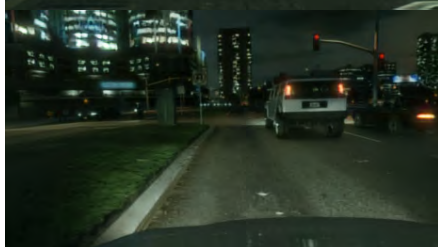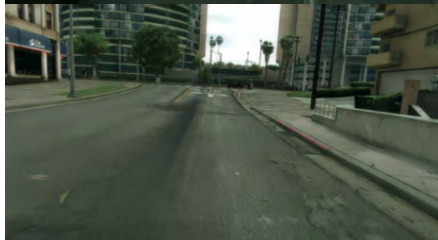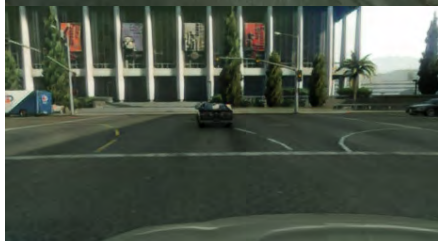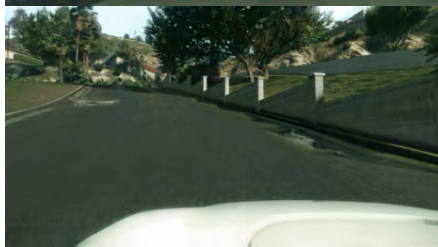

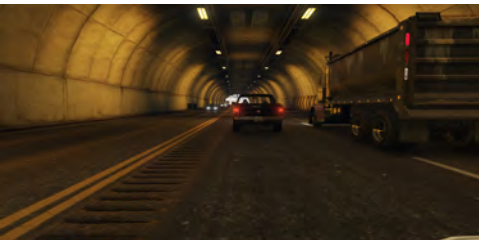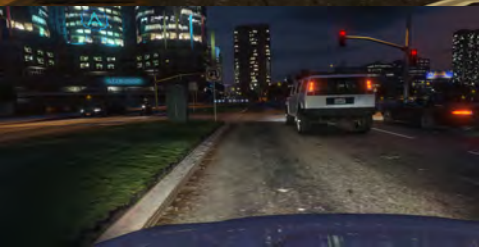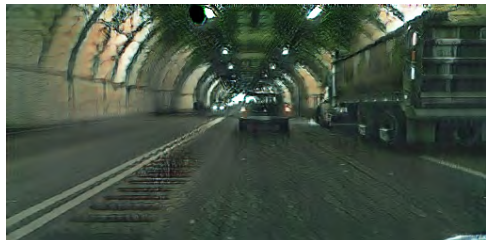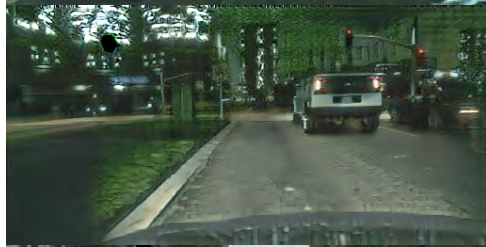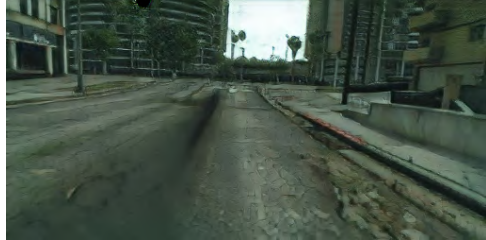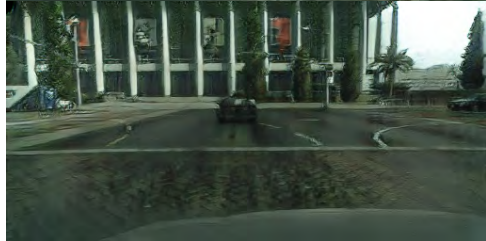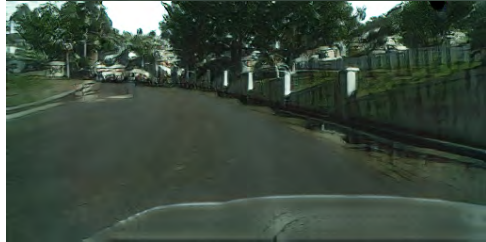

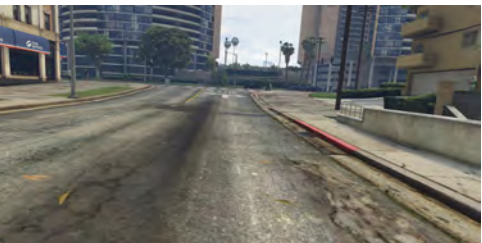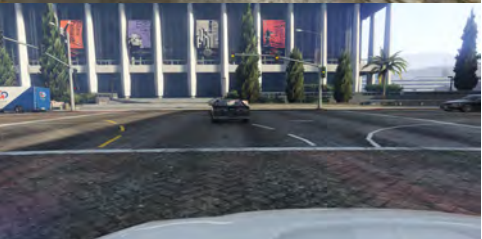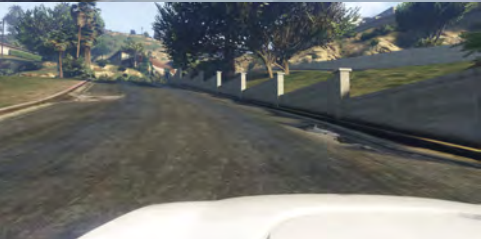



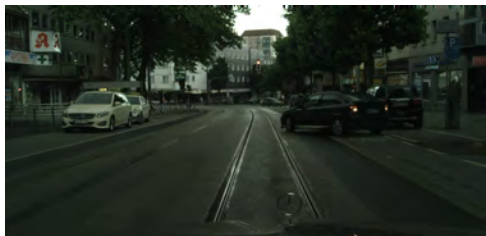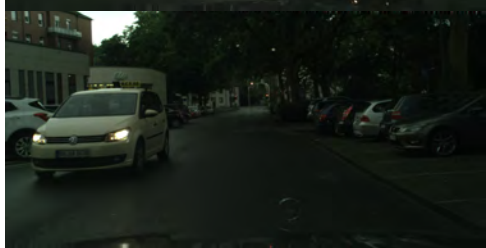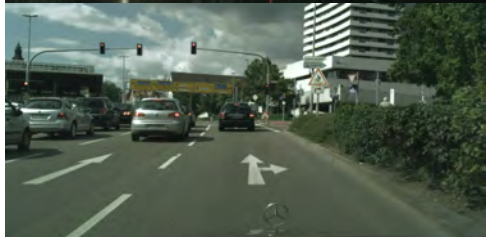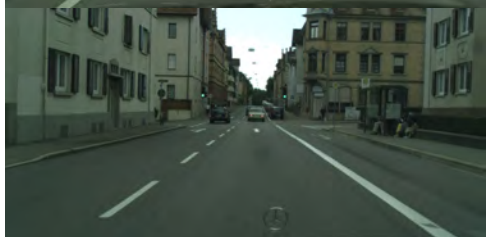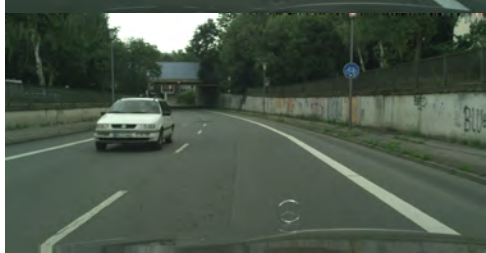

Supplement: Supplementary file 3 [file supplemental_gta_quality.pdf]
